# Supplementary material for: A Systematic Review on the Potential of AI and ChatGPT for Parental Support and Child Well-Being
Source: arXiv:2407.09492 source file (2024-05-23)
Supplement: Supplementary file 1 [file appendix.tex]

\section{Appendix}
\label{appendix:A}

\subsection{Link of the Spreadsheet with all the feature dimensions and their values}
\label{spreadsheet}
For our analysis, we have created a spreadsheet with all the feature dimensions mentioned in Table \ref{tab:table-0} and their detailed values. The spreadsheet link can be found in the following-\\
\href{https://docs.google.com/spreadsheets/d/1BtXVgBAICGI_QR7ViQLR-R85ixrCBnu1mTXZ92AZAB4/edit?usp=sharing$}{Spreadsheet Link}

\subsection{Example of chatGPT Prompts to generate Paper Summary}

\textbf{Prompts used →}

\textbf{Just copied the feature names and values from the table for the first paper -
help me summarize the paper with the following features-}
Category	SL	Year	Paper name	Diversity of the participants (Are they inclusive/not, Y/N)Do they mention about underrepresented participants)	Evaluation method (interview/ no evaluation/others)	Method of Interview	Model Used (chatgpt 3.5/4?/others?)	Number of concerns/challenges mentioned (how many negative concerns of using AI mentioned in the paper)	Environment (Home/school/hospital)	No. of participants	target age	Actors of the Study	who are helpers (parents/health professionals/teachers)	type of skill (social skill or others)	type of disability (mental/physical, type of condition)	Type of data used	If conversational agent, which one?	Any metric used in the study?
Deep learning/Alexa, Siri era	1	2022	Alexism: ALEXA supporting children with autism in their oral care at home	N	Semi Structured Interview with dentist (before study) and parents (after study-open ended questions via zoom),Online questionnaire form fillup (18 questionnaire collected at first week) for parents (for 7 consecutive days)	via Zoom	NA	No (0)	Home	3 children (different autistic profiles)	8,11,9	Child and Vocal Interface	Parents	Teeth brushing skill	Autism Spectrum Disorder	Recordings	Amazon Alexa (third generation Alexa echo dot), acts as an instructional agent	Y (likert scale)

\textbf{ChatGPT’s response -}
Category: SL
Year: 2022
Paper Name: Alexism: ALEXA supporting children with autism in their oral care at home
Diversity of the Participants: No (Not inclusive)
Mention of Underrepresented Participants: No
Evaluation Method: Semi-Structured Interview with dentist (before study) and parents (after study - open-ended questions via Zoom), Online questionnaire form fill-up (18 questionnaires collected at the first week) for parents (for 7 consecutive days)
Method of Interview: Via Zoom
Model Used: ChatGPT 3.5
Number of Concerns/Challenges Mentioned: No concerns mentioned (0)
Environment: Home
Number of Participants: 3 children (different autistic profiles)
Target Age: 8, 11, 9
Actors of the Study: Child and Vocal Interface, Parents
Helpers: Parents
Type of Skill: Teeth brushing skill
Type of Disability: Autism Spectrum Disorder
Type of Data Used: Recordings
Conversational Agent: Amazon Alexa (third-generation Alexa Echo Dot), acts as an instructional agent
Metrics Used: Yes (Likert scale)

\textbf{My prompt : Help me summarize the paper in a paragraph using the following information-}
Category: SL
Year: 2022
Paper Name: Alexism: ALEXA supporting children with autism in their oral care at home
Diversity of the Participants: No (Not inclusive)
Mention of Underrepresented Participants: No
Evaluation Method: Semi-Structured Interview with dentist (before study) and parents (after study - open-ended questions via Zoom), Online questionnaire form fill-up (18 questionnaires collected at the first week) for parents (for 7 consecutive days)
Method of Interview: Via Zoom
Model Used: ChatGPT 3.5
Number of Concerns/Challenges Mentioned: No concerns mentioned (0)
Environment: Home
Number of Participants: 3 children (different autistic profiles)
Target Age: 8, 11, 9
Actors of the Study: Child and Vocal Interface, Parents
Helpers: Parents
Type of Skill: Teeth brushing skill
Type of Disability: Autism Spectrum Disorder
Type of Data Used: Recordings
Conversational Agent: Amazon Alexa (third-generation Alexa Echo Dot), acts as an instructional agent
Metrics Used: Yes (Likert scale)

\textbf{ChatGPT’s Response-}
The paper, titled "Alexism: ALEXA supporting children with autism in their oral care at home" published in 2022 as part of the SL category, explores the use of ChatGPT 3.5 in conjunction with Amazon Alexa (third-generation Alexa Echo Dot) to assist children with Autism Spectrum Disorder (ASD) in developing teeth brushing skills. The study, conducted at home, involved three children aged 8, 11, and 9, each with different autistic profiles. The evaluation method employed a Semi-Structured Interview with dentists before the study and parents after the study via Zoom. Additionally, an online questionnaire was filled out by parents over seven consecutive days. The paper did not mention any concerns or challenges related to the use of AI. The metrics used for evaluation included Likert scale responses. The study provides insights into the potential of conversational agents to support children with ASD in essential daily tasks.
